# Supplementary material for: Effects of training machine-learning potentials for radiation damage simulations using different pseudopotentials
Source: arXiv:2509.11813 source file (2025-09-15)
Supplement: Supplementary file 1 [file supplementary.pdf]

# Supplemental material for: Effects of training machine-learning potentials for radiation damage simulations using different pseudo-potentials.

A. Fellman,<sup>1,\*</sup> J. Byggmästar,<sup>1</sup> F. Granberg,<sup>1</sup> F. Djurabekova,<sup>1</sup> and K. Nordlund<sup>1</sup>

<sup>1</sup>*Department of Physics, P.O. Box 43, FI-00014 University of Helsinki, Finland*

(Dated: September 15, 2025)

## S1. HYPERPARAMETER

There are a multitude of hyperparameters that need to be set when training a GAP model and therefore also tabGAP model. The hyperparameters for the descriptors are given in Table S1. Another set of hyperparameters are the regularisation terms  $\sigma$  for the energies, forces and virials. The default values for these parameters were 1 meV/atom, 0.04 eV Å<sup>-1</sup> and 0.1 eV, respectively. For systems such as liquid structures, dense structures, and short-range interactions (including trajectories) these regularisation terms were increased by a factor of ten ( $10\sigma$ ). The number of grid points used in the tabulation was chosen after convergence testing to be 5000 for both two-body and EAM descriptors and for the three-body grid to be  $80 \times 80 \times 80$ .

TABLE S1: Hyperparameters used for the different descriptors: cutoff radius  $r_{\text{cut}}$ , width of the cutoff region  $r_{\Delta\text{cut}}$ , energy prefactor  $\delta$ , and the number of sparse descriptor environments from the training structures  $M$ .

| Formalism | Descriptor | $r_{\text{cut}}$ (Å) | $r_{\Delta\text{cut}}$ (Å) | $\delta$ | $M$ |
|-----------|------------|----------------------|----------------------------|----------|-----|
| tabGAP    | 2b         | 5.2                  | 1.0                        | 10       | 20  |
|           | EAM        | 5.2                  | 1.0                        | 1.0      | 20  |
|           | 3b         | 4.0                  | 0.6                        | 1.0      | 700 |

## S2. TRAINING DATABASE DESCRIPTION

The original training database included 1457 structures and the recomputed database included 1375 structures. This means that in total 82 structures failed to converge during recalculation with the new VASP parameters. The training data consists of the following classes of structures:

- Randomly distorted unit cells (FCC, BCC and HCP).
- FCC, BCC and HCP lattices at finite temperatures and different volumes, initially created by running MD simulations with earlier iterations of the final potentials.
- Systems containing various small vacancy and interstitial clusters (from one to three defects with different configurations).
- Liquid systems with various densities prepared by melting MD simulations.
- (100), (110) and (111) FCC surfaces.
- Structures with a few disordered surface layers.
- Stacking-fault-like structures where a small slab is moved on a atom plane randomly.
- Dimers and trimers with various distances between atoms.
- Short-range systems, where an atom is randomly inserted into an FCC lattice fairly close to other atoms ( $\geq 1$  Å).
- Structures with trajectories of a single atom being moved along a rigid path in various high-symmetry directions, while the other atoms remained fixed. These are essentially quasi-static drag systems and includes atoms at close distances.

---

\* Corresponding author; aslak.fellman@helsinki.fi

### S3. MODIFICATION OF REPULSIVE POTENTIALS

The parameters of joining ( $r_c$  and  $r_d$ ) where 1.5 and 0.2 for the  $Ni_{reppot}$  and  $Ni_{merged}$  modified potentials.  $Ni_{pvsoft}$  used 1.5 and 0.4 respectively.

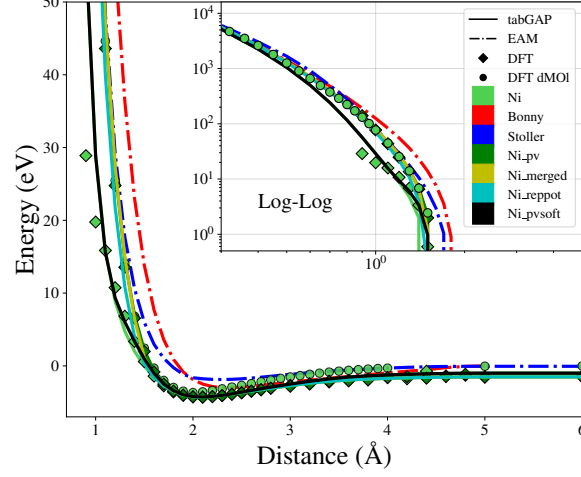

FIG. S1: Dimer curves calculated with the different potentials as well as EAM potentials compared with DFT and all electron DFT used in external repulsive potential.

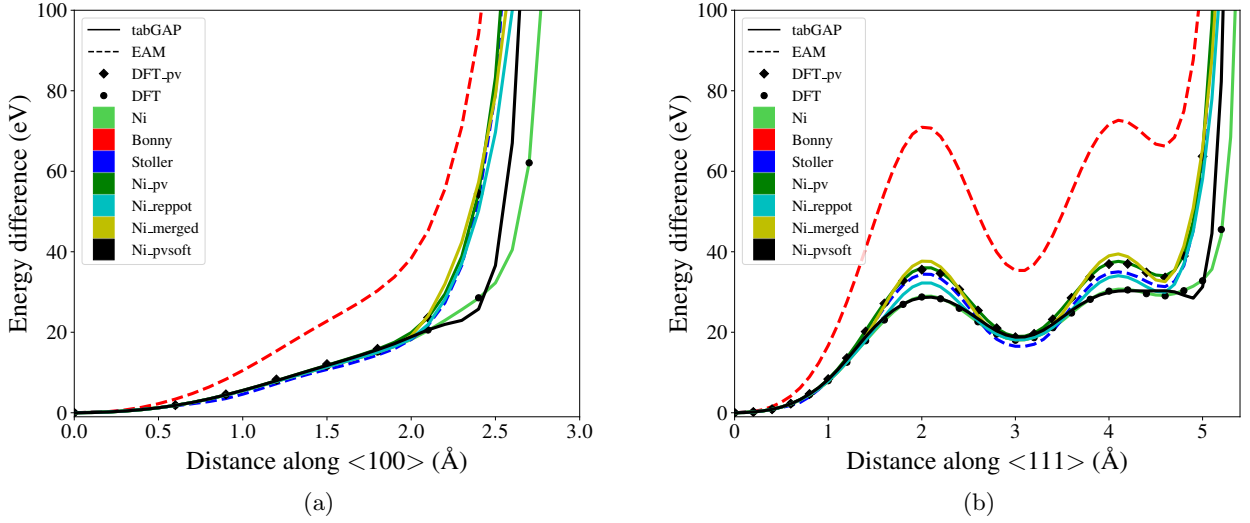

FIG. S2: Total energy difference when displacing a single atom in different high symmetry directions while holding the other atoms stationary.

#### S4. GENERALIZED STACKING FAULT ENERGY CURVE

The generalised stacking fault energy (GSFE) curves shown in Fig. S3, were calculated by displacing one of the  $\{111\}$  slip planes in a  $\langle 112 \rangle$  direction. DFT from Ref. [1].

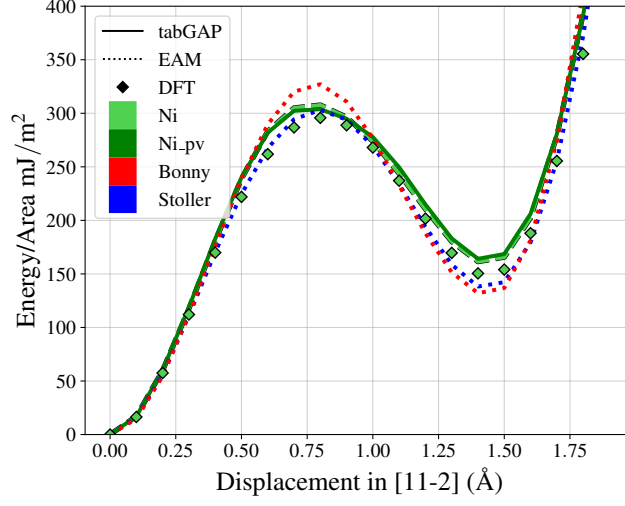

FIG. S3: Generalised stacking fault energy curves calculated with the different potentials and DFT.

#### S5. PHONON DISPERSION

We also calculated the phonon dispersion curves for nickel and compared with the available experimental measurements, as shown in Fig. S4.

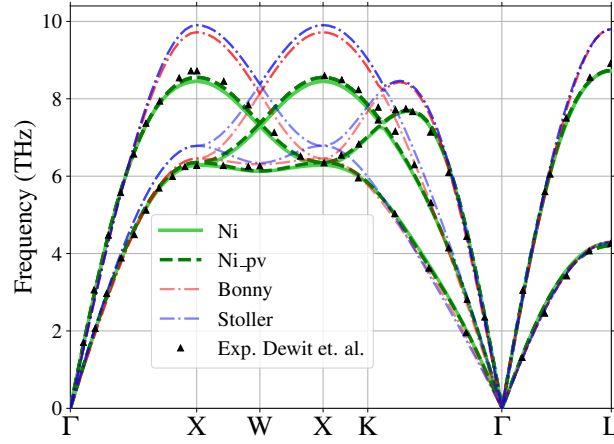

FIG. S4: Phonon dispersion curves calculated using the small displacement method compared to experimental results [2].

## S6. PRIMARY RADIATION DAMAGE

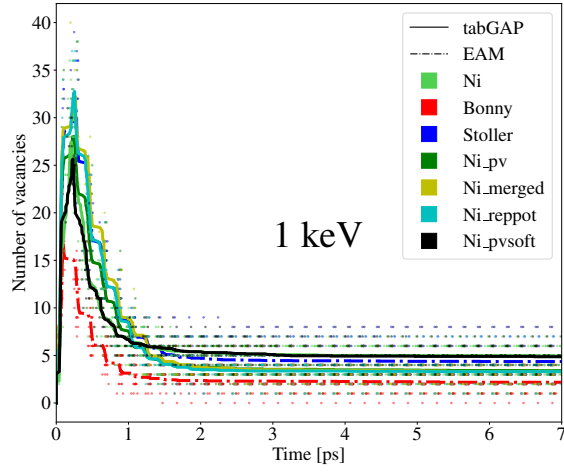

(a) 1 keV

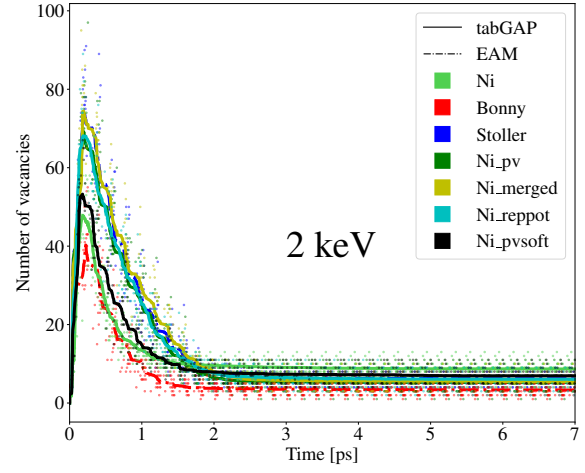

(b) 2 keV

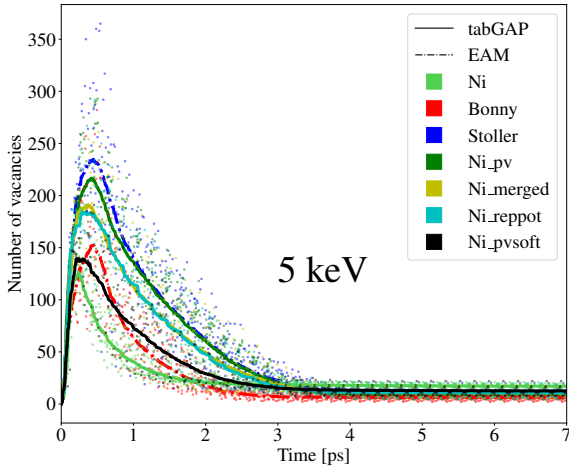

(c) 5 keV

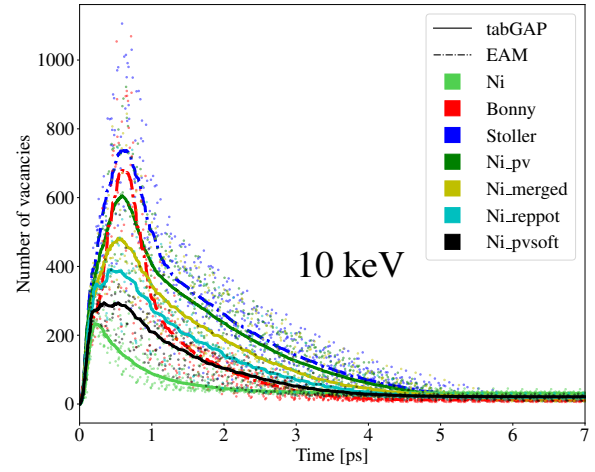

(d) 10 keV

FIG. S5: Number of produced vacancies (from WS analysis) during single cascades as a function of time in different Ni potentials. The curves shown are rolling averages of all the individual cascades together.

## S7. OVERLAPPING CASCADES

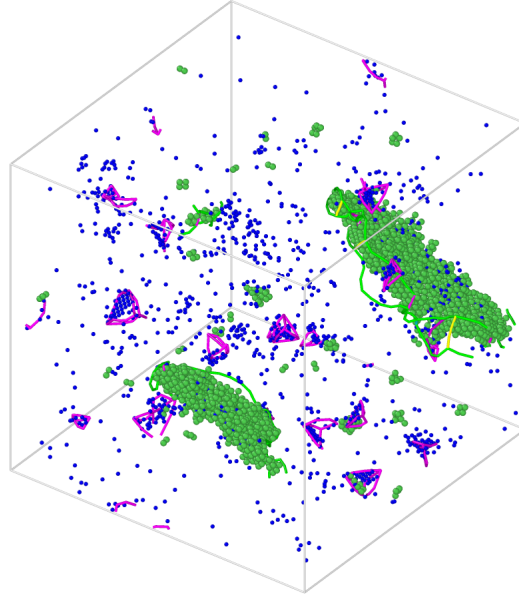

FIG. S6: Final configuration after 4000 overlapping collision cascades with semicore Ni<sub>pv</sub> tabGAP potential. Blue spheres represent vacancies, Green spheres represent interstitial atoms, green lines represent Shockley dislocations, and cyan lines represent Frank dislocations and pink lines represent stair-rod dislocations.

## S8. MODIFIED DEPTH PROFILE RBS/C CALCULATIONS

We investigate the effect of shifting the nuclear energy deposition profile deeper into the sample. This was done by defining a skew normal distributions  $f(x, a, loc)$  to original profile in a manner that the integral under the curve is the same as for the original profile. We use the following equation.  $h * f(x, a, loc)$ , where  $x = r/w$ ,  $h$  is a scaling factor,  $w$  is a width,  $a$  is the skewness and  $loc$  is the shift.

TABLE S2: parameters of the skew normal distributions

| profile     | $h$  | $a$ | $loc$ | $w$  |
|-------------|------|-----|-------|------|
| synthetic   | 3.0  | 1.5 | 0.45  | 4500 |
| synthetic-2 | 3.06 | 1.0 | 0.6   | 4500 |
| synthetic-3 | 3.48 | 0.3 | 1.1   | 4000 |

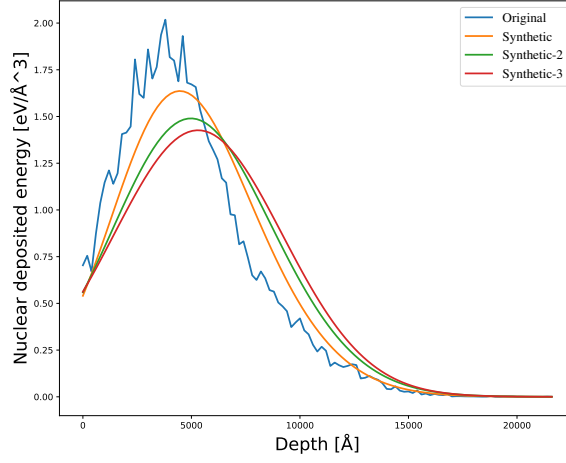

FIG. S7: synthetic nuclear energy deposition profiles. Original profile shows the new calculations of the nuclear energy deposition profiles used in hte manuscript. The  $\theta = 2$  to  $4$  and  $\phi = 0^\circ$  case.

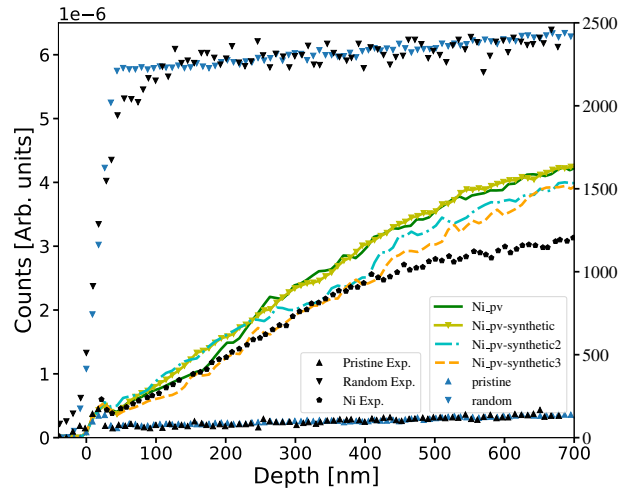

FIG. S8: Comparison between simulated and experimental RBS/c spectra at 300K. Experimental results from Ref. [3]. Simulated structures sampled using nuclear deposited energy profiles show in Fig S7.

- 
- [1] A. Fellman, J. Byggmästar, F. Granberg, K. Nordlund, and F. Djurabekova, Fast and accurate machine-learned inter-atomic potentials for large-scale simulations of Cu, Al and Ni (2024), arXiv:2408.15779 [cond-mat.mtrl-sci].
  - [2] G. DeWit and B. Brockhouse, The lattice dynamics of ferromagnetic and paramagnetic nickel, *Journal of Applied Physics* **39**, 451 (1968).
  - [3] Y. Zhang, G. M. Stocks, K. Jin, C. Lu, H. Bei, B. C. Sales, L. Wang, L. K. Beland, R. E. Stoller, G. D. Samolyuk, M. Caro, A. Caro, and W. J. Weber, Influence of chemical disorder on energy dissipation and defect evolution in concentrated solid solution alloys, *Nature communications* **6** (2015).
